# Supplementary material for: Learning from Spatio-temporal Correlation for Semi-Supervised LiDAR Semantic Segmentation
Source: arXiv:2410.06893 source file (2024-10-09)
Supplement: Supplementary file 1 [file 6_supple.tex]

\clearpage

\appendix

\setcounter{section}{0}
\setcounter{table}{0}
\setcounter{figure}{0}
% \section{Rationale}
% \label{sec:rationale}
% % 
% Having the supplementary compiled together with the main paper means that:
% % 
% \begin{itemize}
% \item The supplementary can back-reference sections of the main paper, for example, we can refer to \cref{sec:intro};
% \item The main paper can forward reference sub-sections within the supplementary explicitly (e.g. referring to a particular experiment); 
% \item When submitted to arXiv, the supplementary will already included at the end of the paper.
% \end{itemize}
% % 
% To split the supplementary pages from the main paper, you can use \href{https://support.apple.com/en-ca/guide/preview/prvw11793/mac#:~:text=Delete%20a%20page%20from%20a,or%20choose%20Edit%20%3E%20Delete).}{Preview (on macOS)}, \href{https://www.adobe.com/acrobat/how-to/delete-pages-from-pdf.html#:~:text=Choose%20%E2%80%9CTools%E2%80%9D%20%3E%20%E2%80%9COrganize,or%20pages%20from%20the%20file.}{Adobe Acrobat} (on all OSs), as well as \href{https://superuser.com/questions/517986/is-it-possible-to-delete-some-pages-of-a-pdf-document}{command line tools}.

% TODO

% Ablation studies on nuScenes as done on SemanticKITTI
% nuScenes
% 1. data statistics
% PLE-lable vs. teacher output
% PLE-label according to time interval
% Qualitative examples

% ScribbleKITTI
% PLE-lable vs. teacher output
% PLE-label according to time interval
% Qualitative examples

% SemanticKITTI Per-class IoU
% nuScenes Per-class IoU
% ScribbleKITTI Per-class IoU

% \tableofcontents

\section{Additional Implementation Details}

This section provides more explanation and technical details for the proposed method.

\subsection{Proximity-based Label Estimation}

We elaborate on the detailed process of proximity-based label estimation (PLE) and provide the pseudo-code in Alg~\ref{alg:PLE}. Our method accommodates multiple labeled scans for each target unlabeled scan. Specifically, within 1-second intervals, we search for the nearest labeled scans, allowing for up to four for SemanticKITTI~\cite{behley2019semantickitti} and one for nuScenes~\cite{caesar2020nuscenes} due to differences in scanning frequency. Then, we transform the coordinates of the labeled scans into the coordinate system of the target unlabeled scan. As mentioned in Sec.~{3.2}, this transformation relies on the pose information provided with LiDAR data, which includes sensor positions during data acquisition. Since the information is relative to the position of the first frame, we calculate the pose difference matrix using pose information between the referenced labeled scan and the target unlabeled scan. The subsequent steps, including proximate point identification and label assignment, align with the process described in Sec.~{3.2}.

\begin{algorithm}[!t]
    \caption{: Pseudo-code for Proximity-based Label Estimation (in NumPy style)}
   \label{alg:PLE}
\begin{algorithmic}[1]
  % \footnotesize
    \small
   \State {\bfseries Input:} Target unlabeled sample $x_k$, Surrounding frame indices $I$, Unlabeled set $X_u$, Labeled set $(X_l, Y_l)$, Pose matrix $P$, Maximum number of reference frames $M$
   
    \State $X_m, Y_m \gets [], []$
    % \STATE $Y_m \gets []$
    
    \For{$i$ $\in$ $I$}
        \If{$\text{len($X_m$)}> M$} 
            \State \text{break} %\Comment{\textit{if there is enough frames, then stop}}
        \EndIf
        \If{$x_j \in X_u$} 
            \State \text{continue} %\Comment{\textit{if unlabeled sample keep searching}}
        \EndIf
        \State $x_i, y_i \gets X_l[i], Y_l[i]$
        % \STATE $y_i \gets Y_l[i]$
        %\Comment{\textit{get homogeneous coordinate}}
        \State $p \gets \text{np.ones}(x_i.\text{shape}[i], 4)$
        \State $p[:, :3] \gets x_i[:, :3]$
        
        \Comment{\textit{Coordinate transform}}
        \State $F \gets \text{np.matmul}(\text{inv}(P_k), P_i)$
        \State $p \gets \text{np.matmul}(F, p^T)^T$
        
        \State $X_m.\text{append}(p)$
        \State $Y_m.\text{append}(y_i)$
    \EndFor
        
    \State $X_m, Y_m \gets \text{concat}(X_m), \text{concat}(Y_m)$
    % \STATE $Y_m \gets $
    
    \State $\text{coord1} \gets x_k[:, :3]$
    \State $\text{coord2} \gets X_m[:, :3]$

    \Comment{\textit{Proximate point identification}}
    \State $\text{kdtree} \gets \text{KDTree}(\text{coord2})$
    \State $\text{dist}, \text{indices} \gets \text{kdtree}.\text{query}(\text{coord1})$

    \Comment{\textit{Label assignment}}
    \State $y_k \gets Y_m[\text{indices}]$
%    \FOR{$b = 1$ \TO $B$}
%    \STATE $x^{(2b-1)}_\text{mix}$, $x^{(2b)}_\text{mix}$ = LaserMix($x^{(b)}_l$, $x^{(b)}_u$) \COMMENT{\textit{LaserMix data}} \\
%    \ENDFOR
%    \STATE $X_\text{mix} = \{{x}^{(i)}_\text{mix}; i \in (1, \ldots, 2B)\}$ 
%    \STATE $S_l$, $S_u$, $S_\text{mix}$ = Student$\big($Concat($X_l$, $X_u$, $X_\text{mix}$)$\big)$ \COMMENT{\textit{Student pred}} \\
%    \STATE $\hat{S}_l$, $\hat{S}_u$ = Teacher$\big($Concat($X_l$, $X_u$)$\big)$  \COMMENT{\textit{Teacher pred}} \\
%    \STATE $Y_u$ = PseudoLabel($\hat{S}_u$, $T$) 
%    \COMMENT{\textit{Pseudo-label generation process}} \\
%    \FOR{$b = 1$ \TO $B$}
%    \STATE $y^{(2b-1)}_\text{mix}$, $y^{(2b)}_\text{mix}$ = LaserMix($y^{(b)}_l$, $y^{(b)}_u$) \COMMENT{\textit{LaserMix label}}\\
%    \ENDFOR
%    \STATE $Y_\text{mix} = \{{y}^{(i)}_\text{mix}; i \in (1, \ldots, 2B)\}$
%    \STATE $L_\text{sup}$ = CrossEntropy($S_l$, $Y_l$) \COMMENT{\textit{Supervised loss}}\\
%    \STATE $L_\text{mix}$ = CrossEntropy($S_\text{mix}$, $Y_\text{mix}$) \COMMENT{\textit{Mixing loss}}\\
%    \STATE $L_\text{mt}$ = L2$\big($Concat($S_l$,  $S_u$), Concat($\hat{S}_l$, $\hat{S}_u$)$\big)$ \COMMENT{\textit{MeanTeacher loss}}\\
%    \STATE ${L} = {L}_{\text{sup}} + \lambda_\textrm{mix} {L}_{\text{mix}} + \lambda_\textrm{mt}{L}_{\text{mt}}$ \COMMENT{\textit{Overall loss}}\\
%    \STATE Backward({L}), Update(Student), UpdateEMA(Teacher) \\
\end{algorithmic}
\end{algorithm}

\subsection{Dual-branch}
We utilize Cylinder3D~\cite{zhou2020cylinder3d} as the backbone network and introduce a dual-branch to the last layer of Cylinder3D. Specifically, we replace a single layer with two parallel sparse convolution layers~\cite{graham2015sparse}. This simple modification segregates the noisy pseudo labels generated by the Teacher network from the accurate ground-truth. Also, it breaks the detrimental training cycle between the pseudo-labels and the Teacher network.

\subsection{Model Configuration}
We adopt Cylinder3D as the backbone network, following the settings of previous work~\cite{kong2023lasermix}. Unlike the original Cylinder3D, which uses a voxel resolution of [480, 360, 32], LaserMix adopts a smaller voxel resolution of  [240, 180, 20]. This modification reduces memory consumption and improves training speed. With this modification, the fully supervised model achieves 58.5\% and 75.2\% mIoU on SemanticKITTI and nuScenes, respectively (see Tab.~{3}). 

\subsection{Training Configuration}
We adopt AdamW~\cite{loshchilov2017decoupled} as the optimizer and use the OneCycle learning rate scheduler~\cite{smith2019super}, following the previous work~\cite{kong2023lasermix}. The maximum learning rate is 0.001, and we use batch sizes of 4 and 8. We train for a total of $45$K iterations. We set the value of $\lambda$ to 250 for the coefficient of $\mathcal{L}_{mt}$.

\section{Additional Experimental Results}

\subsection{Statistics of PLE labels}

Tab.~\ref{sup:tab_ple_kitti} represents the changes in training data statistics and the performance of PLE labels across all labeled ratios on SemanticKITTI~\cite{behley2019semantickitti}. As the ratio of labeled samples increases, the number of samples with either ground-truth or PLE labels also increases. Surprisingly, at a 50\% labeled ratio, all unlabeled samples receive PLE labels. Also, the quality of PLE labels improves as the labeled ratio increases. This is because the referenced labeled scan becomes closer to the target unlabeled scan. 

A similar trend is observed with PLE labels on nuScenes, as detailed in Tab.~\ref{sup:tab_ple_nusc}. The number of remaining unlabeled samples consistently decreases after PLE. Additionally, PLE labels exhibit comparably high quality even in low-budget scenarios, with minimal difference from a normal budget scenario.

% 각 table 값에 대한 해설, 

% \input{sec/tex/supp_tab_component_nusc}
\subsection{Component Analysis}
In Tab.~\ref{sup:component_nusc}, we study the effectiveness of each component in our method across various labeled ratios on nuScenes. The results demonstrate that both PLE and the dual-branch significantly contribute to the performance gains. PLE enhances performance by providing labels with higher accuracy and consistency than pseudo-labels generated by the Teacher network. Meanwhile, the dual-branch effectively enhances performance compared to the baseline, with a more noticeable improvement at lower ratios. This demonstrates the efficacy of the dual-branch in low-budget scenarios. Combining both components further enhances the performance due to their complementary effect. PLE labels augment the amount of data trained with highly accurate labels, while the dual-branch facilitates the training of the remaining unlabeled data without disrupting the training of the C-branch (i.e., clean branch).

\subsection{Class-wise Performance}
Tab.~\ref{sup:classwise_kitti} shows the class-wise IoUs on the \textit{val} set of SemanticKITTI. We compare our method with MeanTeacher~\cite{tarvainen2017mean} and LaserMix~\cite{kong2023lasermix}. Our method demonstrates an overall performance improvement across various classes, particularly evident in dynamic classes. Substantial improvements are observed for \textit{bicycle, motorcycle}, and \textit{pedestrian} across all ratios, while \textit{bicyclist} and \textit{bus} exhibit moderate improvements in the majority of ratios. These classes may occupy a small portion of the dataset, but they are crucial in autonomous driving scenarios. The significant improvement in these dynamic classes demonstrates the effectiveness of our method in real-world applications. Additionally, our method exhibits moderate improvements in static classes such as \textit{vegetation}, \textit{trunk}, \textit{terrain}, and \textit{pole}. 

Similarly, class-wise performance on the \textit{val} set of nuScenes shown in Tab.~\ref{sup:classwise_nusc} follows a similar trend. Our method exhibits significant performance improvements in dynamic classes such as \textit{bicycle, motorcycle}, and \textit{pedestrian}. Additionally, we observe moderate performance improvements in classes such as \textit{truck, construction vehicle, traffic cone}, and \textit{trailer}, either across all ratios or in the majority of cases. We speculate that PLE is different from the conventional pseudo-labeling, which is prone to overfitting to majority classes~\cite{wang2022semi}, as it is capable of generating accurate labels for the minor classes.

% 잘하는 클래스 언급 & 그 클래스들이 자율주행 시나리오에서 중요하다

\subsection{Qualitative Examples}

We present qualitative results on the \textit{val} set of SemanticKITTI in a bird's-eye view, as shown in Fig.~\ref{sup:qualitative_kitti}. Correct predictions are marked in light gray, while errors are marked in red. We highlight the areas where our method (LaserMix + Ours) outperforms LaserMix with dashed circles. The qualitative examples exhibit consistent results with the class-wise performance. Specifically, our method accurately identifies \textit{pedestrian} and \textit{bicyclist} classes, as shown in the 1st and 3rd rows. Moreover, in the 2nd and 4th rows, our method exhibits superior accuracy in recognizing \textit{truck} and \textit{bicycle} classes when compared to LaserMix. These results emphasize the effectiveness of our method in precisely recognizing classes in driving scenarios.

Qualitative results on the \textit{val} set of nuScenes exhibit a similar tendency as illustrated in Fig.~\ref{sup:qualitative_nusc}. Firstly, our method excels in identifying the \textit{pedestrian} class, indicating a strong capability in recognizing person-related classes (1st row). Moreover, our method exhibits proficiency in identifying various vehicle-related classes, including \textit{car, bus} and \textit{truck} (2nd-4th rows). Particularly, our method effectively identifies \textit{car} and \textit{bus} objects close to the ego vehicle, as shown in the 2nd and 3rd rows. These results support the efficacy of our method in autonomous scenarios, showcasing its applicability in real-world autonomous environments.
% Caption에 있는 클래스/row 별로 언급하기
